# Supplementary material for: Vision Transformer for NeRF-Based View Synthesis from a Single Input Image
Source: arXiv:2207.05736 source file (2022-10-13)
Supplement: Supplementary file 1 [file ablation.tex]

\section{Extra Results for Ablation Studies}\label{sec:ablation_extra}

For the modified sampling strategy mentioned in Sec.~\ref{sec:implementation}, we tested the visual quality without this strategy and it shows worse results with incorrect geometry in Fig.~\ref{fig:ablation}, proving that it is better to utilize the modified sampling strategy.

\begin{figure}[t]
\centering
\includegraphics[width=1.0\textwidth]{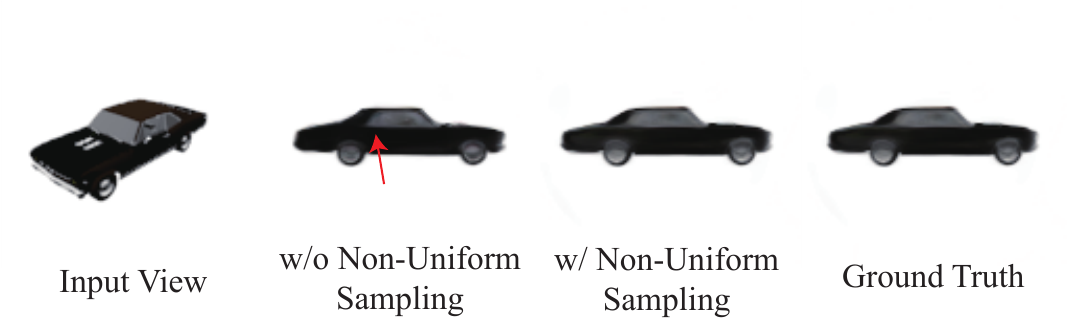}
\caption{\boldstart{Ablation studies on sampling strategy.}}
\label{fig:ablation}
\end{figure}
