# Supplementary material for: Vision Transformer for NeRF-Based View Synthesis from a Single Input Image
Source: arXiv:2207.05736 source file (2022-10-13)
Supplement: Supplementary file 2 [file category_agnostic.tex]

\section{Extra Results for Category-Agnostic View Synthesis}

We show additional qualitative results on category-agnostic view synthesis in Fig.~\ref{fig:nmr_1} and ~\ref{fig:nmr_2}.
Our proposed method achieves better quality across all categories than PixelNeRF.
Note that the structures and fine details are better synthesized in our rendered images, even in occluded regions.

\begin{figure}[t]
\centering
\includegraphics[width=1.0\textwidth]{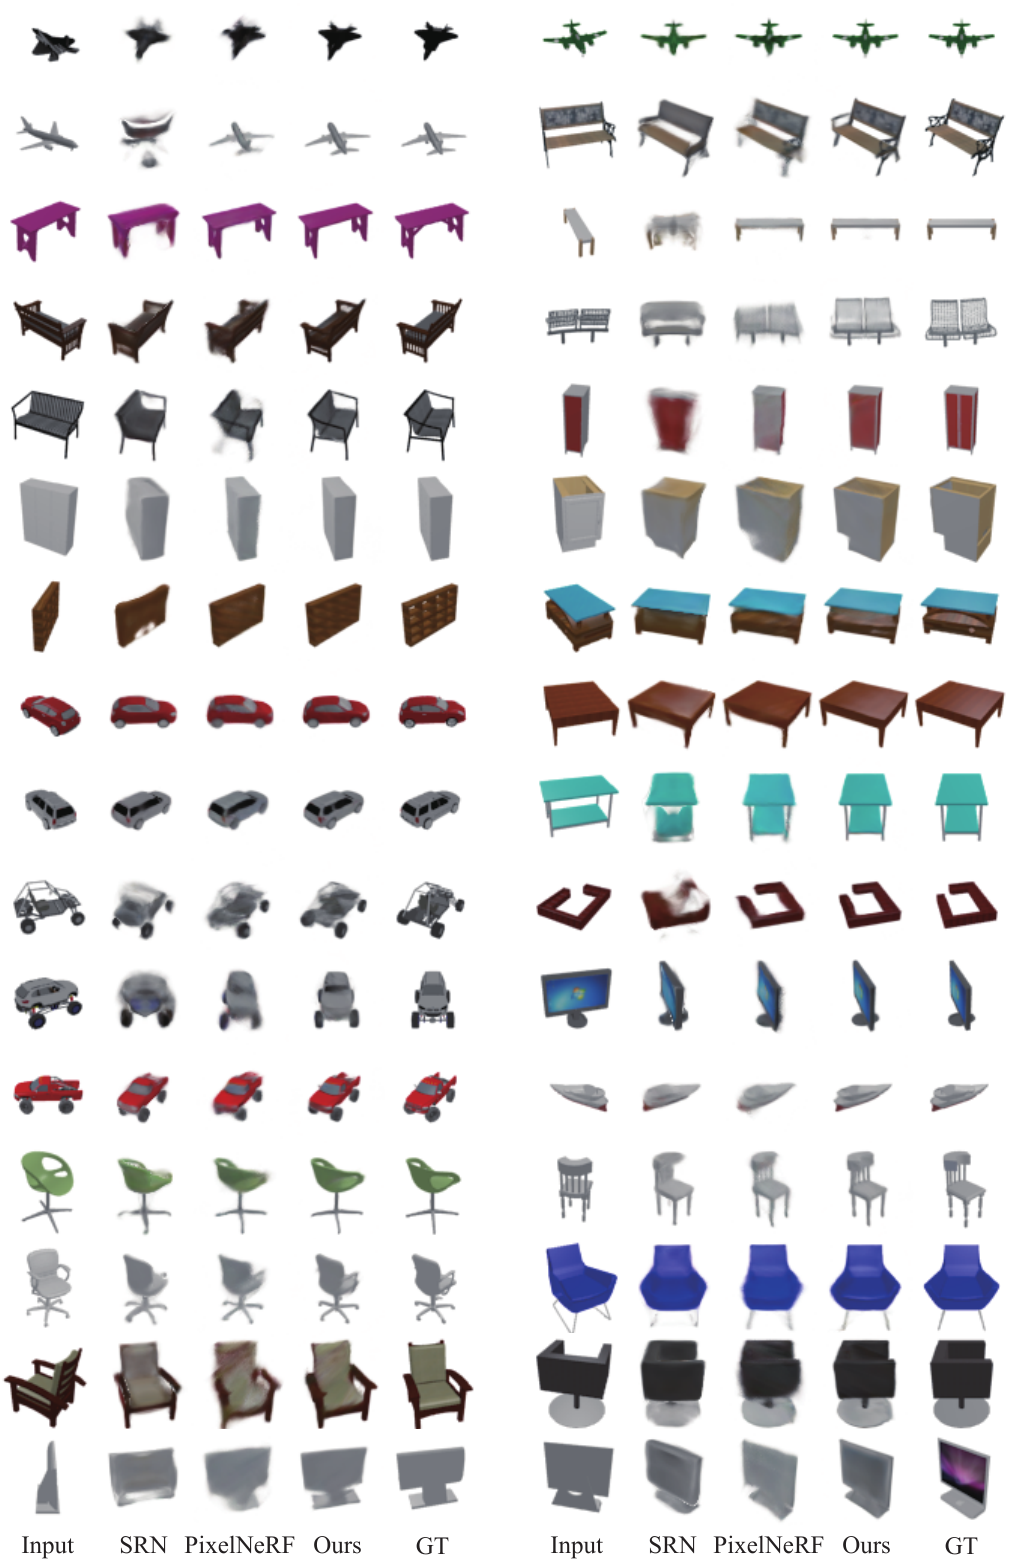}
\caption{\boldstart{Category-agnostic view synthesis results.} }
\label{fig:nmr_1}
\end{figure}

\begin{figure}[t]
\centering
\includegraphics[width=1.0\textwidth]{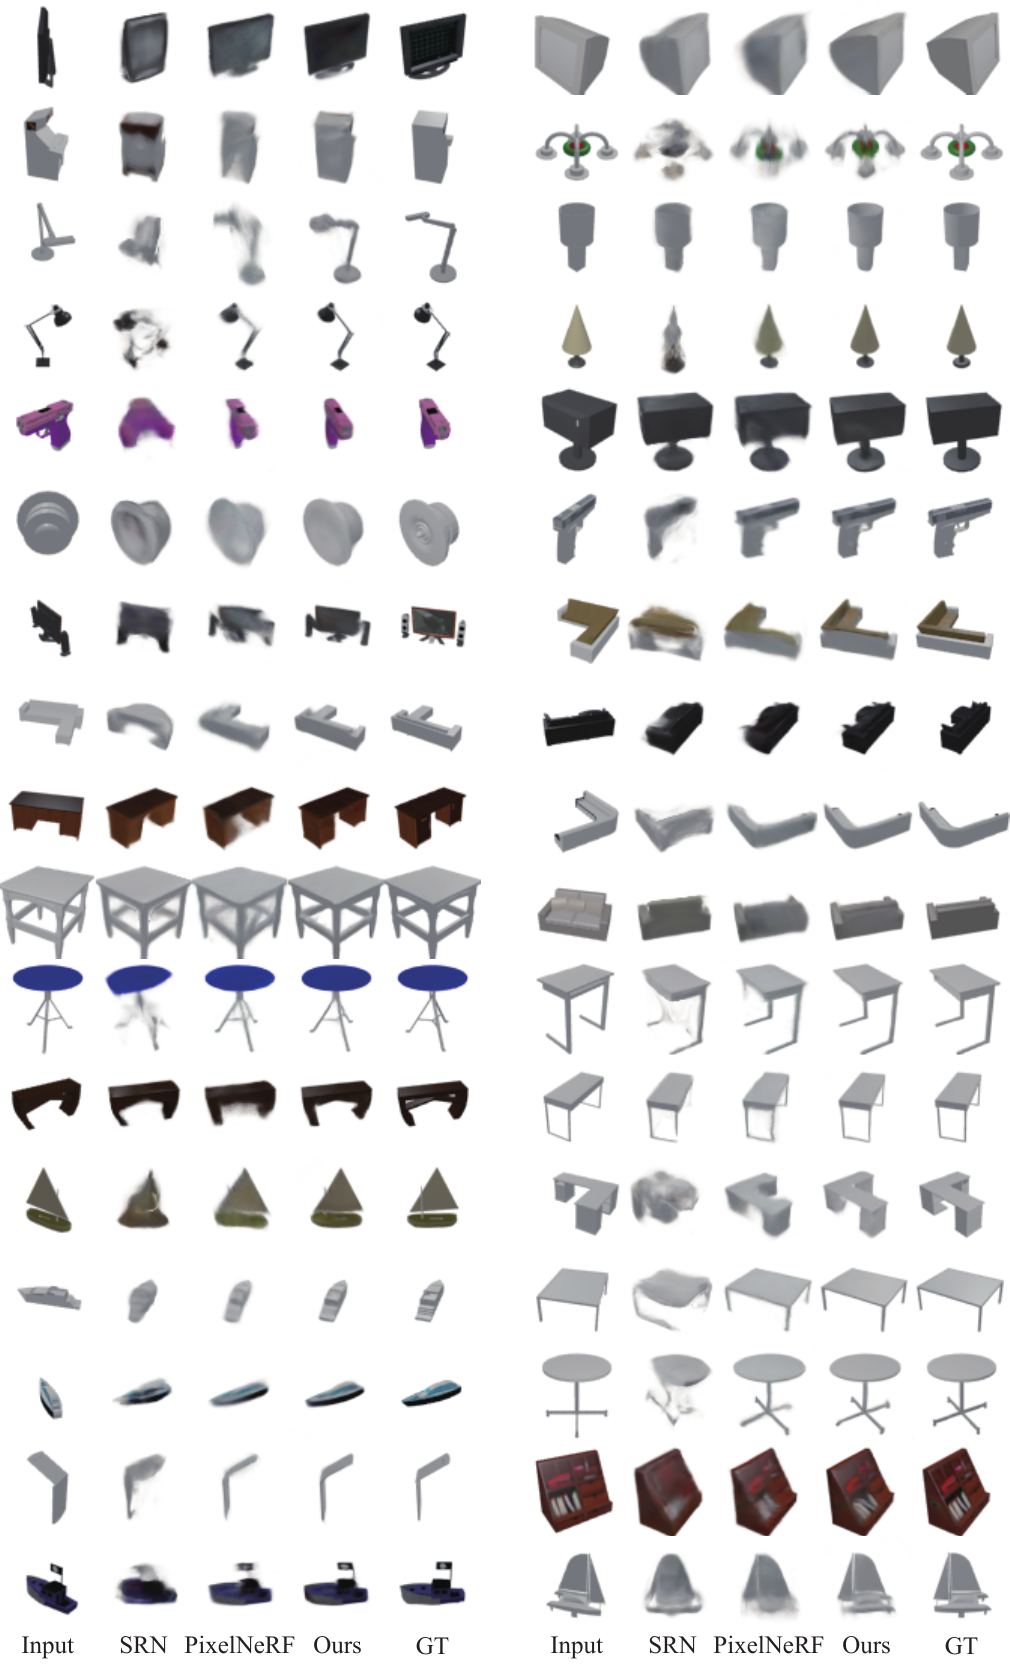}
\caption{\boldstart{Additional category-agnostic view synthesis results.} }
\label{fig:nmr_2}
\end{figure}
